# Supplementary material for: Learning to Solve Complex Problems via Dataset Decomposition
Source: arXiv:2602.20296 source file (2026-02-23)
Supplement: Supplementary file 1 [file aime_appendix.tex]

AIME 2024-II-4

\begin{longtable}{@{}p{\textwidth}@{}}
\caption{\textbf{\data{} sample stemming from s1-prob.} The black text is the question and the \textcolor{olmoeDarkYellow}{yellow} text is the solution. Based solely on the question we generate the \textcolor{defaultlightblue}{light blue} reasoning trace and \textcolor{defaultblue}{blue} response with Gemini, which we use for training.} 
\label{tab:prob} \\
\toprule

Question: Let $x,y$ and $z$ be positive real numbers that satisfy the following system of equations:$\log_2(\frac{x}{yz}) = \frac{1}{2}$$\log_2(\frac{y}{xz}) = \frac{1}{3}$$\log_2(\frac{z}{xy}) = \frac{1}{4}$. Then the value of $\left|\log_2(x^4y^3z^2)\right|$ is $\frac{m}{n}$ where $m$ and $n$ are relatively prime positive integers. Find $m+n$. \\

Solution: Denote $\log_2(x) = a$, $\log_2(y) = b$, and $\log_2(z) = c$.
Then, we have:$a-b-c = \frac{1}{2}$,$-a+b-c = \frac{1}{3}$,$-a-b+c = \frac{1}{4}$.
Now, we can solve to get $a = \frac{-7}{24}$, $b = \frac{-9}{24}$, $c = \frac{-5}{12}$.
Plugging these values in, we obtain $|4a + 3b + 2c| = \frac{25}{8}$ $\implies \boxed{33}$.

\\

\defaultyellow{

Question: Simplify the fraction $\frac{-9}{24}$ and express it in its simplest form.} \\
\defaultyellow{ 
Solution: To simplify the fraction $\frac{-9}{24}$, we need to find the greatest common divisor (GCD) of the numerator and the denominator. First, we find the prime factors of each number: - The prime factors of 9 are $3 \times 3$. - The prime factors of 24 are $2 \times 2 \times 2 \times 3$. The common prime factor is 3. Next, we divide both the numerator and the denominator by their GCD, which is 3: $\frac{-9 \div 3}{24 \div 3} = \frac{-3}{8}$. Therefore, the fraction $\frac{-9}{24}$ simplified is $\frac{-3}{8}$.

%\begin{enumerate}
%\item    "a": "-3/8",
%\item    "depth": 1,
%\item    "tags": "\"Fraction Simplification\"",
%\item  "cot": "To simplify the fraction $\frac{-9}{24}$, we need to find the greatest common divisor (GCD) of the numerator and the denominator. First, we find the prime factors of each number: - The prime factors of 9 are $3 \times 3$. - The prime factors of 24 are $2 \times 2 \times 2 \times 3$. The common prime factor is 3. Next, we divide both the numerator and the denominator by their GCD, which is 3: $\frac{-9 \div 3}{24 \div 3} = \frac{-3}{8}$. Therefore, the fraction $\frac{-9}{24}$ simplified is $\frac{-3}{8}$."
%\end{enumerate}

} \\

\defaultyellow{Question: What is the greatest common divisor (GCD) of -9 and 24?}\\
\defaultyellow{
Solution: To find the greatest common divisor (GCD) of -9 and 24, we first consider the absolute values of the numbers, which are 9 and 24. The GCD is the largest positive integer that divides both numbers without leaving a remainder. 1. List the factors of 9: 1, 3, 9. 2. List the factors of 24: 1, 2, 3, 4, 6, 8, 12, 24 3. Identify the common factors: 1, 3. 4. The greatest common factor is 3. Thus, the GCD of -9 and 24 is 3.}

\defaultyellow{What is the greatest common divisor (GCD) of the numbers 9 and 24, based on their prime factorizations?}
\defaultyellow{To find the greatest common divisor (GCD) of 9 and 24, we first determine their prime factorizations: - The prime factorization of 9 is $3 \times 3$. - The prime factorization of 24 is $2 \times 2 \times 2 \times 3$. Next, we identify the common prime factors. Both numbers share the prime factor 3. The highest power of the common prime factor 3 that appears in both factorizations is $3^1$. Therefore, the GCD of 9 and 24 is 3.}

\\

\defaultlightblue{

\begin{enumerate}
\item Question: What is the greatest common divisor (GCD) of -9 and 24?
    Solution: "To find the greatest common divisor (GCD) of -9 and 24, we first consider the absolute values of the numbers, which are 9 and 24. The GCD is the largest positive integer that divides both numbers without leaving a remainder. 1. List the factors of 9: 1, 3, 9. 2. List the factors of 24: 1, 2, 3, 4, 6, 8, 12, 24 3. Identify the common factors: 1, 3. 4. The greatest common factor is 3. Thus, the GCD of -9 and 24 is 3.",
    "a": "3",
    "depth": 2,
    "tags": "GCD Calculation"
\end{enumerate}
\begin{enumerate}
"q": "What is the greatest common divisor (GCD) of the numbers 9 and 24, based on their prime factorizations?",
    "cot": "To find the greatest common divisor (GCD) of 9 and 24, we first determine their prime factorizations: - The prime factorization of 9 is $3 \times 3$. - The prime factorization of 24 is $2 \times 2 \times 2 \times 3$. Next, we identify the common prime factors. Both numbers share the prime factor 3. The highest power of the common prime factor 3 that appears in both factorizations is $3^1$. Therefore, the GCD of 9 and 24 is 3.",
    "a": "3",
    "depth": 2,
    "tags": "Prime Factorization"
\end{enumerate}

\begin{enumerate}
    "q": "What is the greatest common divisor (GCD) of the numbers -9 and 24 using their prime factorizations?",
    "cot": "To find the greatest common divisor (GCD) of -9 and 24, we first need to determine the prime factorizations of each number.
    1. Prime factorization of -9:
    - The number 9 can be factored into prime numbers as follows: $9 = 3 \times 3$.
    - Since -9 is simply 9 with a negative sign, the prime factorization of -9 is $-1 \times 3 \times 3$.
    2. Prime factorization of 24:  - The number 24 can be factored into prime numbers as follows: $24 = 2 \times 12$.
    - Breaking down 12 further: $12 = 2 \times 6$.  - Breaking down 6 further: $6 = 2 \times 3$.
    - Combining these, the prime factorization of 24 is $2 \times 2 \times 2 \times 3$ or $2^3 \times 3$.
    3. Identifying common prime factors:  
    - The prime factors of -9 are $-1, 3, 3$.   
    - The prime factors of 24 are $2, 2, 2, 3$.   
    - The common prime factor between -9 and 24 is 3. 4. Calculating the GCD:  
    - The only common prime factor is 3, and it appears once in both factorizations. 
    - Therefore, the GCD of -9 and 24 is 3.",
    "a": "3",
    "depth": 2,
    "tags": "Prime Factorization"
\end{enumerate}

\begin{enumerate}
{
    "q": "Simplify the fraction $\frac{-12}{32}$ and express it in its simplest form.",
    "cot": "To simplify the fraction $\frac{-12}{32}$, we need to find the greatest common divisor (GCD) of the numerator and the denominator. 
    1. The factors of 12 are: 1, 2, 3, 4, 6, 12.
    2. The factors of 32 are: 1, 2, 4, 8, 16, 32.
    3. The common factors of 12 and 32 are: 1, 2, 4.
    4. The greatest common divisor (GCD) is 4.
    Next, we divide both the numerator and the denominator by their GCD, which is 4:
    $\frac{-12 \div 4}{32 \div 4} = \frac{-3}{8}$
    Therefore, the fraction $\frac{-12}{32}$ simplified is $\frac{-3}{8}$.",
    "a": "-3/8",
    "depth": 2,
    "tags": "Simplifying Fractions"
  }
\end{enumerate}

}
\\
\defaultyellow{

\begin{enumerate}
    "q": "Given the equations $4a + 3b + 2c = \frac{25}{8}$, find the value of $|4a + 3b + 2c|$.",
    "a": "25/8",
    "depth": 1,
    "tags": "Absolute Value Equation",
    "cot": "We start with the equation $4a + 3b + 2c = \frac{25}{8}$. To find the absolute value, we take $|4a + 3b + 2c|$. Since $4a + 3b + 2c$ is already given as $\frac{25}{8}$, the absolute value is $|\frac{25}{8}|$. The absolute value of $\frac{25}{8}$ is simply $\frac{25}{8}$ because it is already positive."
\end{enumerate}
}

\defaultblue{
\begin{enumerate}
    "q": "Given the equation $4a + 3b + 2c = \frac{25}{8}$, what is the value of $4a + 3b + 2c$?",
    "cot": "We start with the given linear equation:
    $4a + 3b + 2c = \frac{25}{8}$
    The equation directly states that the value of the expression $4a + 3b + 2c$ is $\frac{25}{8}$. Therefore, no further calculations are needed.",
    "a": "25/8",
    "depth": 2,
    "tags": "Linear Equation"
\end{enumerate}

\begin{enumerate}
    "q": "Given the equation $4a + 3b + 2c = \frac{25}{8}$, find the value of $|4a + 3b + 2c|$.",
    "cot": "To find the absolute value of the expression $4a + 3b + 2c$, we start with the given equation:
    $4a + 3b + 2c = \frac{25}{8}$
    The absolute value of a number is the non-negative value of that number without regard to its sign. Therefore, we need to find the absolute value of $\frac{25}{8}$:
    $|4a + 3b + 2c| = \left|\frac{25}{8}\right|$
    Since $\frac{25}{8}$ is already a positive number, its absolute value is the same as the number itself:
    $\left|\frac{25}{8}\right| = \frac{25}{8}$
    Thus, the value of $|4a + 3b + 2c|$ is $\frac{25}{8}$.",
    "a": "25/8",
    "depth": 2,
    "tags": "Absolute Value Calculation"
\end{enumerate}

{
    "q": "Given the equation $4a + 3b + 2c = \frac{25}{8}$, what is the absolute value of $4a + 3b + 2c$?",
    "cot": "1. The equation $4a + 3b + 2c = \frac{25}{8}$ is given.
    2. To find the absolute value of $4a + 3b + 2c$, we take the absolute value of the right-hand side of the equation.
    3. The right-hand side of the equation is $\frac{25}{8}$.
    4. The absolute value of $\frac{25}{8}$ is $|\frac{25}{8}|$.
    5. Since $\frac{25}{8}$ is a positive number, its absolute value is simply $\frac{25}{8}$.",
    "a": "25/8",
    "depth": 2,
    "tags": "Absolute Value Calculation"
  },

  {
    "q": "What is the absolute value of $\frac{25}{8}$?",
    "cot": "To find the absolute value of a number, we consider its distance from zero on the number line, which is always a non-negative value. The given number is $\frac{25}{8}$.
    Step 1: Determine if the number is positive or negative.
    - $\frac{25}{8}$ is a positive number.
    Step 2: Since the number is already positive, its absolute value is the number itself.
    Therefore, the absolute value of $\frac{25}{8}$ is $\frac{25}{8}$.",
    "a": "25/8",
    "depth": 2,
    "tags": "Absolute Value"
  }

  }
\\
\bottomrule
\end{longtable}
